# Supplementary material for: Finite-temperature conductivity and magnetoconductivity of topological insulators
Source: arXiv:1312.0385 source file (2014-04-08)
Supplement: Supplementary file 1 [file Supplemental_Material.pdf]

# Supplemental Material
# for
# “Finite-temperature conductivity and magnetoconductivity of topological insulators”

Hai-Zhou Lu and Shun-Qing Shen
*Department of Physics, The University of Hong Kong, Pokfulam Road, Hong Kong, China*
(Dated: March 7, 2014)

**Contents**

**S1. Conductivity formulae.** 1
A. Semiclassical conductivity $\sigma^{sc}$. 1
B. Conductivity correction from quantum interference $\sigma^{qi}$. 2
C. Conductivity correction from electron-electron interaction $\sigma^{ee}$. 3
D. Summary of defined weight factors and length corrections 4
E. Conductivity formula in different limits of $B$ and $T$ 5
1. Limit $B \to 0$ or $T \to \infty$ 5
2. Limit $B \to \infty$ or $T \to 0$ 5

**S2. An introduction of the calculation.** 6
A. Interaction-induced conductivity correction. 6
B. Dynamically screened chiral interaction. 8
C. Disorder scattering. 8
D. Diffuson and Cooperon. 9
E. In magnetic field. 9

**S3. Screening factor $F$.** 10

**S4. Conductivity for $\Delta/2E_F$ between 0 and 1.** 12

**S5. Slope of $\sigma$ vs. $\ln T$.** 12
A. Experimental data of slope. 12
B. Theory of slope. 13

**References** 15

## S1. CONDUCTIVITY FORMULAE.

The total conductivity originally has three parts: the semiclassical conductivity $\sigma^{sc}$, the correction from the quantum interference $\sigma^{qi}$, and the correction from the electron-electron interaction $\sigma^{ee}$. Because $\sigma^{sc}$ does not have temperature and magnetic field dependence, we only discuss $\sigma^{qi}$ and $\sigma^{ee}$ in the main text. For convenience, we define

$$\sigma = \sigma^{qi} + \sigma^{ee}. \tag{S1}$$

### A. Semiclassical conductivity $\sigma^{sc}$.

The semiclassical conductivity is found as

$$\sigma^{sc} = e^2 N_F D, \tag{S2}$$

where $-e$ is the electron charge, $N_F = E_F/2\pi\gamma^2$ is the density of states, $E_F$ is the Fermi energy measured from the Dirac point located at the middle of the gap, $\gamma = v\hbar$, $v$ is the effective velocity of the Dirac fermions, $D$ is the diffusion

coefficient. For the massive Dirac fermions,

$$D = \frac{1}{2} v_F^2 \tau \eta_v, \tag{S3}$$

where the Fermi velocity $v_F = v\sqrt{1-(\Delta/2E_F)^2}$, $\tau$ is the momentum relaxation time, and the vertex correction to the velocity[1] for the massive Dirac fermions[2] is found as

$$\eta_v = [1 - a^2 b^2/(a^4+b^4)]^{-1}, \tag{S4}$$

where $a \equiv \cos(\theta/2) = \sqrt{(1+\Delta/2E_F)/2}$, $b \equiv \sin(\theta/2) = \sqrt{(1-\Delta/2E_F)/2}$, and $\cos\theta \equiv \Delta/2E_F$.

In this work, we use $\ell$, the mean free path, as the parameter to derive $\tau$ and $D$. By definition, $\ell^2 = D\tau$, so $\ell^2 = v_F^2 \tau^2 \eta_v/2$, or

$$\tau = \frac{\ell}{v_F}\sqrt{\frac{2}{\eta_v}}, \quad D = \ell v_F \sqrt{\frac{\eta_v}{2}}. \tag{S5}$$

### B. Conductivity correction from quantum interference $\sigma^{qi}$.

At zero magnetic field, the conductivity correction from the quantum interference is found as[2]

$$\sigma^{qi}(B=0,T) = \frac{e^2}{\pi h}\sum_{i=0,1}\alpha_i \ln\frac{\ell^2}{\ell_{\phi i}^2}, \tag{S6}$$

where $e^2/h$ is the conductance quantum, $\ell$ is the mean free path. The effective phase coherence length for the singlet ($i=1$) and triplet ($i=0$) Cooperons are defined as

$$1/\ell_{\phi i}^2 \equiv 1/\ell_\phi^2 + 1/\ell_i^2 \equiv 1/\ell_\phi^2 + \Omega_i/D_i, \tag{S7}$$

$D_i$ and $\Omega_i$ are the diffusion coefficents and gaps of the Cooperons (see Sec. S2 D) defined as

$$\begin{aligned} D_0 &= \frac{1}{2}v_F^2\tau(1+\frac{1}{g_1}), \quad \Omega_0 = g_0/2\tau, \quad 1/\ell_0^2 \equiv \Omega_0/D_0 = \eta_v g_0/2\ell^2(1+1/g_1), \\ D_1 &= \frac{1}{2}v_F^2\tau(1+\frac{1}{g_0}+\frac{1}{g_2}), \quad \Omega_1 = g_1/2\tau, \quad 1/\ell_1^2 \equiv \Omega_1/D_1 = \eta_v g_1/2\ell^2(1+1/g_0+1/g_2), \end{aligned} \tag{S8}$$

where we have used the relation $\ell^2 \equiv D\tau$, and

$$g_0 = 2\frac{b^4}{a^4}, \quad g_1 = \frac{(a^2-b^2)^2}{a^2b^2}, \quad g_2 = 2\frac{a^4}{b^4}. \tag{S9}$$

Compare to our previous work, we have moved $\sin\theta$ from the definitions of $\ell_0$ and $\ell_1$ to that of $v_F$. As a result, $\ell_0$ and $\ell_1$ diverges in both massless and massive limits (Fig. S1) and where $\ell_{\phi i}$ reduce to $\ell_\phi$, the phase coherence length. $\ell_\phi$ is proportional to $T^{-p/2}$, where $p=1$ ($p=3$) in two-dimensional disordered metals if the electron-electron (electron-phonon) interaction is the main decoherence source[3–5]. $\sigma^{qi}$ describes a crossover between WAL and WL as a function of $\Delta/2E_F$[2], with $\alpha_0$ as the weight factor for WL and $\alpha_1$ for WAL[2],

$$\alpha_1 = -\frac{\eta_v^2(1+2\eta_H)}{2(1+1/g_0+1/g_2)}, \quad \alpha_0 = \frac{\eta_v^2(1+2\eta_H)}{2(1/g_1+1)}, \tag{S10}$$

where $\eta_H$ is from the dressed Hikami boxes and $\eta_H = -(1-1/\eta_v)/2$ or $\eta_v(1+2\eta_H) = 1$ if there is only elastic scattering. According to the values of $\alpha_0$ and $\alpha_1$ in Fig. S1, $\sigma^{qi}$ can be roughly written as

$$\sigma^{qi}(B=0,T) = \frac{e^2}{\pi h}\alpha p \ln\frac{T}{\ell^2}, \tag{S11}$$

up to an overall shift. Here $\alpha$ is a function of $\Delta/2E_F$ for the massive Dirac model. $\alpha = -1/2$ at $\Delta/2E_F = 0$, corresponding to WAL; while $\alpha = 1/2$ as $\Delta/2E_F \to 1$, corresponding to WL. In contrast, for the conventional two-dimensional electron gas (2DEG), $\alpha \in [-1/2, 1]$ is a function of spin-orbit scattering time[7]. In the presence of a perpendicular magnetic field $B$,

$$\sigma^{qi}(B,T) = \frac{e^2}{\pi h}\sum_{i=0,1}\alpha_i\left[\psi(\frac{1}{2}+\frac{\ell_B^2}{\ell_{\phi i}^2}) - \ln\frac{\ell_B^2}{\ell^2}\right], \tag{S12}$$

where $\psi$ is the digamma function and $\ell_B \equiv \sqrt{\hbar/4eB}$ is the magnetic length. The $\psi$ and ln terms in Eq. (S12) cancel in a strong magnetic field, leading to

$$\sigma^{qi}(B \gg B_\phi, T) = 0, \tag{S13}$$

where $B_\phi = \hbar/4e\ell_\phi^2$ is determined by the phase coherence length. A shorter $\ell_\phi$ gives a larger $B_\phi$. The magnetoconductivity can be defined from Eqs. (S6) and (S12)

$$\delta\sigma^{qi}(B,T) \equiv \sigma^{qi}(B,T) - \sigma^{qi}(0,T) = \frac{e^2}{\pi h}\sum_{i=0,1}\alpha_i\left[\psi(\frac{1}{2}+\frac{\ell_B^2}{\ell_{\phi i}^2}) - \ln\frac{\ell_B^2}{\ell_{\phi i}^2}\right]. \tag{S14}$$

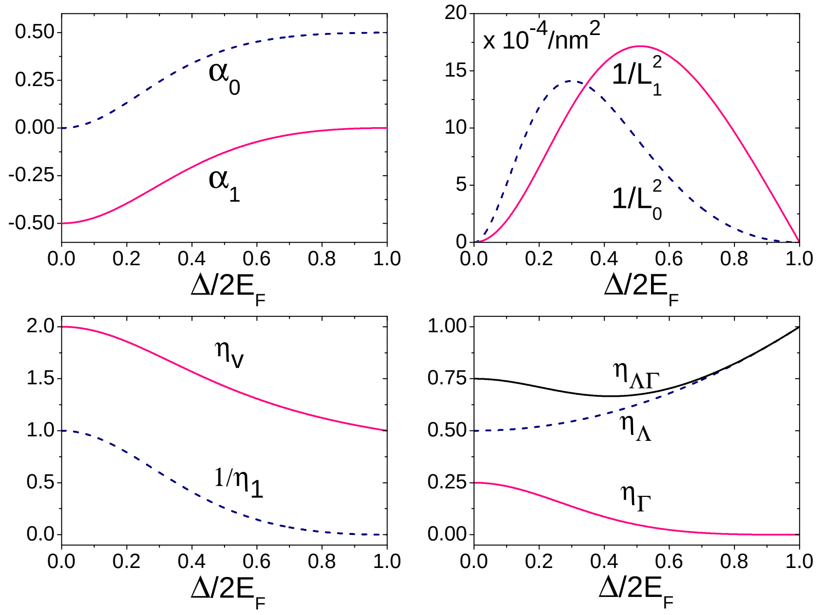


FIG. S1: **Quantities in the conductivity formula as a function of $\Delta/2E_F$.** The gap $\Delta$ is measured by the Fermi energy $E_F$, thus $\Delta/2E_F$ serves as a control parameter. $\alpha_0$ and $\alpha_1$ are weight factors for WL and WAL terms in $\sigma^{qi}$ [Eq. (2) in the main text], respectively[2]. In the main text and Eq. (S11), $\alpha = \alpha_1 = -1/2$ at $\Delta/2E_F = 0$; and $\alpha = \alpha_0 \to 1/2$ as $\Delta/2E_F \to 1$. In this work, $\ell_0$ and $\ell_1$ have different definitions compared to those in our previous work[2], and they diverge in both the massless and large-mass limits. $\eta_v$ is the vertex correction to the velocity[1,2]. $\eta_1$ is defined in Eq. (S19). The weight factor $\eta_\Lambda$ indicates the contribution from the Hartree-Diffuson self-energy and $\eta_\Gamma$ from Hartree-Cooperon and Fork-Cooperon self-energies. In the section **Conductivity formula** of the main text, we have defined $\eta_{\Lambda\Gamma} = \eta_\Lambda + \eta_\Gamma$ [Eq. (3) in the main text], which is 3/4 at $\Delta/2E_F = 0$ and 1 as $\Delta/2E_F \to 1$. Parameters: $\gamma = 3$ eVÅ. $\ell = 10$ nm.

### C. Conductivity correction from electron-electron interaction $\sigma^{ee}$.

The electron-electron interaction can give extra self-energies, which correct the density of states on the Fermi surface, leading to the conductivity correction[3–5]. The leading-order self-energies come from the direct (Hartree) and exchange (Fock) interactions. In contrast to in a clean system, the disorder scattering can give dressed corrections [Fig. S2 (d)], known as the Diffuson (particle-hole correlation) and Cooperon (particle-particle correlation). $\sigma^{ee}$ is calculated from the Fock-Diffuson, Hartree-Diffuson, Fock-Cooperon, and Hartree-Cooperon self-energies.

The conductivity correction from the interaction is found as

$$\sigma^{ee}(T,B) = \frac{e^2}{\pi h}\left[1 - \eta_{\Lambda\Gamma}F\right]\ln\frac{2\ell^2}{\ell_T^2} - \frac{e^2}{\pi h}\eta_\Gamma F\psi\left(\frac{1}{2}+\frac{\ell_T^2}{\ell_{B\phi}^2}\right), \tag{S15}$$

where

$$\eta_{\Lambda\Gamma} = \eta_\Lambda + \eta_\Gamma, \tag{S16}$$

where the weight factor $\eta_\Lambda$ is from the Hartree-Diffuson self-energy and $\eta_\Gamma$ is from Hartree-Cooperon and Fock-Cooperon self-energies, and

$$\begin{aligned}\eta_\Lambda &= a^4+b^4=\frac{1}{2}[1+(\frac{\Delta}{2E_F})^2],\\ \eta_\Gamma &= \frac{a^2b^2}{\eta_1(1-g_1)}\approx\frac{a^2b^2}{\eta_1}=a^2b^2\frac{\eta_v}{(1+1/g_0+1/g_2)}=\frac{1}{4}[1-(\frac{\Delta}{2E_F})^2]\frac{\eta_v}{(1+1/g_0+1/g_2)},\end{aligned} \tag{S17}$$

where the approximation is valid in the vicinity of the massless and large-mass limits. Figure S1 shows that $\eta_\Gamma=1/4$ and $\eta_\Lambda=1/2$ at $\Delta/2E_F=0$; while as $\Delta/2E_F\to 1$, $\eta_\Gamma=0$, $\eta_\Lambda=1$, and $\sigma^{ee}\propto(e^2/\pi h)(1-F)\ln T$, which recovers the 2DEG result[5] calculated from the same diagrams.

In Eq. (S15), $\ell_T\equiv\sqrt{D\hbar/2\pi k_B T}$ is the thermal diffusion length, with $k_B$ the Boltzmann constant and $D$ the diffusion coefficient, and

$$\frac{1}{\ell_{B\phi}^2}=\frac{\eta_1}{2\ell_B^2}+\frac{\eta_1}{\ell_{\phi1}^2}=-\frac{1}{2\alpha_1}(\frac{1}{2\ell_B^2}+\frac{1}{\ell_{\phi1}^2}), \tag{S18}$$

where $\ell_{\phi1}$ has been defined in Eq. (S7) and $\ell_B=\sqrt{\hbar/4eB}$. According to Eqs. (S3) and (S8),

$$\eta_1\equiv D_1/D=\frac{1+1/g_0+1/g_2}{\eta_v}=-\frac{1}{2\alpha_1}. \tag{S19}$$

$1/\eta_1$ as a function of $\Delta/2E_F$ is shown in Fig. S1. The screening factor $F$ will be introduced in Sec. S3 in detail.

The magnetoconductivity $\delta\sigma^{ee}(B)\equiv\sigma^{ee}(T,B)-\sigma^{ee}(T,0)$ can be found from Eq. (S15) as

$$\delta\sigma^{ee}(B)=-\frac{e^2}{\pi h}\eta_\Gamma F\left[\psi\left(\frac{1}{2}+\frac{\ell_T^2}{\ell_{B\phi}^2}\right)-\psi\left(\frac{1}{2}+\frac{\ell_{T1}^2}{\ell_{\phi1}^2}\right)\right], \tag{S20}$$

where

$$\ell_{T1}\equiv\sqrt{\frac{D_1\hbar}{2\pi k_B T}}=\sqrt{\eta_1}\sqrt{\frac{D\hbar}{2\pi k_B T}}=\frac{\ell_T}{\sqrt{-2\alpha_1}}. \tag{S21}$$

### D. Summary of defined weight factors and length corrections

In the conductivity formula Eqs. (2) and (3) of the main text, we have defined weight factors and corrections to lengths

$$\begin{aligned}\alpha_0 &= \frac{1}{2}\frac{(a^4+b^4)(a^2-b^2)^2}{(a^4+b^4-a^2b^2)^2},\quad \alpha_1=-\frac{a^4b^4}{(a^4+b^4)(a^4+b^4-a^2b^2)},\\ \eta_1 &= \frac{(a^4+b^4)(a^4+b^4-a^2b^2)}{2a^4b^4},\quad \eta_v=\frac{a^4+b^4}{a^4+b^4-a^2b^2},\\ \ell_0^2 &= \ell^2\frac{(a^4+b^4-a^2b^2)^2}{(a^4+b^4)(a^2-b^2)^2}\frac{a^4}{b^4},\quad \ell_1^2=\ell^2\frac{(a^4+b^4)(a^4+b^4-a^2b^2)}{a^2b^2(a^2-b^2)^2}.\end{aligned} \tag{S22}$$

Using

$$a^4+b^4=\frac{1}{2}(1+\cos^2\theta),\quad a^2b^2=\frac{1}{4}\sin^2\theta,\quad a^2-b^2=\cos\theta, \tag{S23}$$

the weigh factors

$$\begin{aligned}\alpha_0 &= \frac{4\cos^2\theta(1+\cos^2\theta)}{(1+3\cos^2\theta)^2},\quad \alpha_1=-\frac{1}{2}\frac{\sin^4\theta}{(1+\cos^2\theta)(1+3\cos^2\theta)},\\ \eta_\Gamma &= -\alpha_1\frac{\sin^2\theta}{2},\quad \eta_\Lambda=\frac{1+\cos^2\theta}{2},\quad \eta_{\Lambda\Gamma}=\eta_\Gamma+\eta_\Lambda,\quad \eta_v=\frac{2(1+\cos^2\theta)}{1+3\cos^2\theta},\end{aligned} \tag{S24}$$

and the corrections to lengths

$$\ell_0^2=\ell^2\frac{\cot^4\frac{\theta}{2}}{2\alpha_0},\quad \ell_1^2=-\ell^2\frac{\tan^2\theta}{4\alpha_1},\quad \eta_1=-\frac{1}{2\alpha_1}, \tag{S25}$$

where cot means the cotangent function.

### E. Conductivity formula in different limits of $B$ and $T$

#### 1. Limit $B \to 0$ or $T \to \infty$

In these two limits, $\ell_B \gg \ell_\phi$. Besides, the formula is valid for $\ell \ll \ell_T \ll \ell_\phi$, so the overall relation is

$$\ell \ll \ell_T \ll \ell_\phi \ll \ell_B. \tag{S26}$$

Using $\psi(x) \approx \ln(x) - \frac{1}{2x}$ for $x \to \infty$,

$$\begin{aligned}\sigma^{qi} &= \frac{e^2}{\pi h}\sum_{i=0,1}\alpha_i\left[\psi\left(\frac{1}{2}+\frac{\ell_B^2}{\ell_{\phi i}^2}\right)-\ln\frac{\ell_B^2}{\ell^2}\right] \approx \frac{e^2}{\pi h}\sum_{i=0,1}\alpha_i\left[\ln\frac{\ell_B^2}{\ell_{\phi i}^2}-\frac{\ell_{\phi i}^2}{2\ell_B^2}+\ln\frac{\ell^2}{\ell_B^2}\right]\\ &= \frac{e^2}{\pi h}\sum_{i=0,1}\alpha_i\left[\ln\frac{\ell^2}{\ell_{\phi i}^2}-\frac{\ell_{\phi i}^2}{2\ell_B^2}\right] = \frac{e^2}{\pi h}\sum_{i=0,1}\alpha_i\left[\ln\left(\frac{\ell^2}{\ell_\phi^2}+\frac{\ell^2}{\ell_i^2}\right)-\frac{\ell_{\phi i}^2}{2\ell_B^2}\right],\end{aligned} \tag{S27}$$

and

$$\begin{aligned}\sigma^{ee} &= \frac{e^2}{\pi h}(1-\eta_{\Lambda\Gamma}F)\ln\frac{2\ell^2}{\ell_T^2}-\frac{e^2}{\pi h}\eta_\Gamma F\psi\left[\frac{1}{2}+\frac{1}{2|\alpha_1|}(\frac{\ell_T^2}{2\ell_B^2}+\frac{\ell_T^2}{\ell_{\phi 1}^2})\right]\\ &\approx \frac{e^2}{\pi h}(1-\eta_{\Lambda\Gamma}F)\ln\frac{2\ell^2}{\ell_T^2}-\frac{e^2}{\pi h}\eta_\Gamma F\psi\left[\frac{1}{2}+\frac{1}{2|\alpha_1|}\frac{\ell_T^2}{\ell_{\phi 1}^2}\right].\end{aligned} \tag{S28}$$

Because of $\ell_i$, there is no $\ln T$ dependence for arbitrary mass. In either massless or large-mass limit,

$$\begin{aligned}\sigma^{qi} &\approx \frac{e^2}{\pi h}\alpha\left[\ln\frac{\ell^2}{\ell_\phi^2}-\frac{\ell_\phi^2}{2\ell_B^2}\right] \approx \frac{e^2}{\pi h}\alpha\left[\ln\frac{\ell^2}{CT^{-p}}-\frac{CT^{-p}4eB}{2\hbar}\right]\\ &= \frac{e^2}{\pi h}\left[\alpha p\ln\frac{\ell^2 T}{C}-\alpha\frac{C2eB}{\hbar T^p}\right] = \frac{e^2}{\pi h}\left[\alpha p\ln T-\frac{2\alpha eC}{\hbar}\frac{B}{T^p}+\alpha p\ln\frac{\ell^2}{C}\right],\end{aligned} \tag{S29}$$

so it defines a linear magnetoconductivity

$$\delta\sigma^{qi}(B) \approx -\frac{e^2}{\pi h}\alpha\frac{\ell_\phi^2}{2\ell_B^2} = -\frac{e^2}{h}\frac{2\alpha e\ell_\phi^2}{\pi\hbar}|B|, \tag{S30}$$

where $\alpha = -1/2$ for the massless limit and $\alpha = 1/2$ for the large-mass limit, and

$$\begin{aligned}\sigma^{ee} &\approx \frac{e^2}{\pi h}(1-\eta_{\Lambda\Gamma}F)\ln\frac{2\ell^2}{\ell_T^2}-\frac{e^2}{\pi h}\eta_\Gamma F\psi\left[\frac{1}{2}+\frac{\ell_T^2}{\ell_\phi^2}\right] \approx \frac{e^2}{\pi h}(1-\eta_{\Lambda\Gamma}F)\ln\frac{2\ell^2 2\pi k_B T}{D\hbar}-\frac{e^2}{\pi h}\eta_\Gamma F\psi\left(\frac{1}{2}\right)\\ &\approx \frac{e^2}{\pi h}(1-\eta_{\Lambda\Gamma}F)\ln T+\frac{e^2}{\pi h}(1-\eta_{\Lambda\Gamma}F)\ln\frac{4\pi k_B\ell^2}{D\hbar}-\frac{e^2}{\pi h}\eta_\Gamma F\psi\left(\frac{1}{2}\right),\end{aligned} \tag{S31}$$

where $\eta_{\Lambda\Gamma} = 1/2+1/4 = 3/4$, $\eta_\Gamma = 1/4$ for the massless limit and $\eta_\Gamma = 0$ in the large-mass limit, and $\eta_\Lambda = 1$. When $B = 0$, the slope is given by

$$\kappa \equiv \frac{\pi h}{e^2}\frac{\partial(\sigma^{qi}+\sigma^{ee})}{\partial\ln T} = \alpha p+1-\eta_{\Lambda\Gamma}F. \tag{S32}$$

#### 2. Limit $B \to \infty$ or $T \to 0$

In these two limits, $\ell_B \ll \ell_T, \ell_\phi$, and there is still $\ell \ll \ell_B$ and $\ell \ll \ell_T \ll \ell_\phi$ so the overall relation is

$$\ell \ll \ell_B \ll \ell_T \ll \ell_\phi. \tag{S33}$$

$$\begin{aligned}\sigma^{qi} &= \frac{e^2}{\pi h}\sum_{i=0,1}\alpha_i\left[\psi\left(1/2+\ell_B^2/\ell_{\phi i}^2\right)-\ln(\ell_B^2/\ell^2)\right]\approx\frac{e^2}{\pi h}\sum_{i=0,1}\alpha_i\left[\psi\left(1/2\right)-\ln(\hbar/4eB\ell^2)\right]\\&\approx\frac{e^2}{\pi h}\sum_{i=0,1}\alpha_i\left[\ln B+\ln(4e\ell^2/\hbar)+\psi\left(1/2\right)\right],\end{aligned}\tag{S34}$$

since there is no $\ell_\phi$, $\sigma^{qi}$ has no $T$ dependence in the limit that $B\to\infty$ or $T\to 0$.

$$\begin{aligned}\sigma^{ee} &= \frac{e^2}{\pi h}(1-\eta_{\Lambda\Gamma}F)\ln\frac{2\ell^2}{\ell_T^2}-\frac{e^2}{\pi h}\eta_\Gamma F\psi\left[\frac{1}{2}+\frac{1}{2|\alpha_1|}\left(\frac{\ell_T^2}{2\ell_B^2}+\frac{\ell_T^2}{\ell_{\phi 1}^2}\right)\right]\\&\approx\frac{e^2}{\pi h}(1-\eta_{\Lambda\Gamma}F)\ln\frac{2\ell^2}{\ell_T^2}-\frac{e^2}{\pi h}\eta_\Gamma F\left[\ln\frac{\ell_T^2}{4|\alpha_1|\ell_B^2}-\frac{2|\alpha_1|\ell_B^2}{\ell_T^2}\right]\\&=\frac{e^2}{\pi h}(1-\eta_{\Lambda\Gamma}F)\ln\frac{4\pi k_B\ell^2T}{D\hbar}-\frac{e^2}{\pi h}\eta_\Gamma F\left[\ln\frac{DeB}{|\alpha_1|2\pi k_BT}-\frac{|\alpha_1|\pi k_BT}{eBD}\right]\\&=\frac{e^2}{\pi h}(1-\eta_{\Lambda\Gamma}F)(\ln T+\ln\frac{4\pi k_B\ell^2}{D\hbar})-\frac{e^2}{\pi h}\eta_\Gamma F\left[\ln B-\ln T-\frac{|\alpha_1|\pi k_BT}{eBD}+\ln\frac{De}{|\alpha_1|2\pi k_B}\right]\\&\approx\frac{e^2}{\pi h}(1-\eta_\Lambda F-\eta_\Gamma F)(\ln T+\ln\frac{4\pi k_B\ell^2}{D\hbar})-\frac{e^2}{\pi h}\eta_\Gamma F\left[\ln B-\ln T+\ln\frac{De}{|\alpha_1|2\pi k_B}\right]\\&=\frac{e^2}{\pi h}(1-\eta_\Lambda F)(\ln T+\ln\frac{4\pi k_B\ell^2}{D\hbar})-\frac{e^2}{\pi h}\eta_\Gamma F(\ln B+\ln\frac{De}{|\alpha_1|2\pi k_B}),\end{aligned}\tag{S35}$$

where $\eta_\Gamma\ln T$ terms are cancelled because they are from the Cooperon, which can be destroyed by the magnetic field. When $B\to\infty$,

$$\kappa\equiv\frac{\pi h}{e^2}\frac{\partial(\sigma^{qi}+\sigma^{ee})}{\partial\ln T}=1-\eta_\Lambda F.\tag{S36}$$

## S2. AN INTRODUCTION OF THE CALCULATION.

The procedure to calculate the semiclassical conductivity $\sigma^{sc}$ and the conductivity correction from the quantum interference $\sigma^{qi}$ has been introduced in our previous works[2,8,9]. Here, we only introduce how to calculate $\sigma^{ee}$.

### A. Interaction-induced conductivity correction.

The conductivity correction from the electron-electron interaction is found from

$$\sigma^{ee}=\sigma^{sc}\frac{\delta N(0)}{N_F},\tag{S37}$$

where $N_F=E_F/2\pi\gamma^2$ is the density of states at the Fermi energy $E_F$, $\sigma^{sc}=e^2N_FD$ is the semiclassical conductivity. The diffusion coefficient is found as

$$D=\frac{1}{2}v_F^2\tau\eta_v,\tag{S38}$$

where the Fermi velocity $v_F=(\gamma/\hbar)\sqrt{1-(\Delta/2E_F)^2}$, and the vertex correction to the velocity[1] for the massive Dirac fermions[2] is found as

$$\eta_v=[1-a^2b^2/(a^4+b^4)]^{-1}.\tag{S39}$$

The change of the density of states on the Fermi surface $\delta N(0)$ due to the interaction can be found from[3]

$$\delta N(\epsilon)=-\frac{1}{\pi}\mathrm{Im}\sum_{\mathbf{k}}[\mathcal{G}^2(\mathbf{k},\epsilon_n)\Sigma_{ee}(\mathbf{k},\epsilon_n)]_{i\epsilon_n\to\epsilon+i0^+},\tag{S40}$$

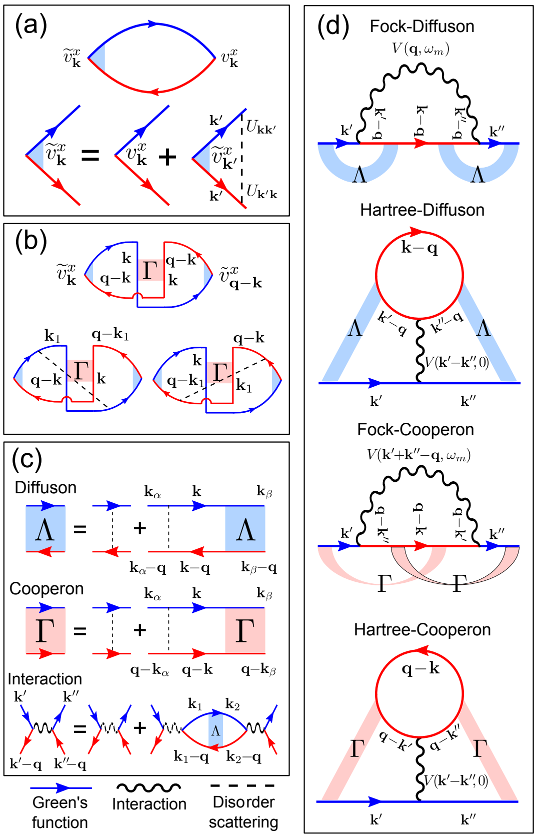


FIG. S2: (a) The diagram for the semiclassical conductivity $\sigma^{sc}$. $v$ and $\tilde{v}$ are the bare velocity and the velocity after the vertex correction, respectively. (b) The Hikami boxes of the maximally-crossed diagrams, from which the conductivity correction from the quantum interference $\sigma^{qi}$ is calculated.[6] (c) The iteration equations for the Diffuson ($\Lambda$), Cooperon ($\Gamma$), and dynamically screened interaction. (d) The Fock and Hartree self-energies dressed by Diffuson and Cooperon, from which the conductivity correction from the electron-electron interaction $\sigma^{ee}$ is calculated. $\mathbf{k}$ and $\mathbf{q}$ stand for the wave vectors, $\epsilon_n$ and $\omega_m$ for the Matsubara frequencies.

where $\Sigma_{ee}$ is the self-energy from the electron-electron interaction, $\mathcal{G}$ is the Matsubara Green function dressed by the disorder scattering under the Born approximation

$$\mathcal{G}_{\mathbf{k}}^{\epsilon_n} \equiv \mathcal{G}(\mathbf{k}, \epsilon_n) = \frac{1}{i\hbar\epsilon_n - \xi_{\mathbf{k}} + i(\hbar/2\tau)\mathrm{sgn}(\epsilon_n)}, \tag{S41}$$

where $\epsilon_n = (2n+1)\pi k_B T/\hbar$ is the Fermionic frequency ($n \in \mathbb{Z}$), $\xi_{\mathbf{k}} = \epsilon_{\mathbf{k}} - E_F$, $\epsilon_{\mathbf{k}} = \sqrt{(\Delta/2)^2 + \gamma^2 k^2}$ is the dispersion of the upper energy band of the massive Dirac model, $k^2 = k_x^2 + k_y^2$. The self-energy $\Sigma_{ee} = \Sigma_\Lambda^{\mathrm{F}} + \Sigma_\Lambda^{\mathrm{H}} + \Sigma_\Gamma^{\mathrm{F}} + \Sigma_\Gamma^{\mathrm{H}}$ are calculated from the diagrams in Fig. S2 (d), with $\Lambda$ for the Diffuson, $\Gamma$ for Cooperon, F for Fock, and H for Hartree. We give two examples

$$\begin{aligned}
\Sigma_\Lambda^{\mathrm{F}}(\mathbf{k}, \epsilon_n) &= -\frac{1}{\beta}\sum_{\omega_m}\sum_{\mathbf{q}}\sum_{\mathbf{k}'}\sum_{\mathbf{k}''} V_{\mathbf{k}''-\mathbf{q}\to\mathbf{k}''}^{\mathbf{k}'\to\mathbf{k}'-\mathbf{q}} \Lambda(\mathbf{k}, \mathbf{k}', \omega_m)\Lambda(\mathbf{k}'', \mathbf{k}, \omega_m)\mathcal{G}_{\mathbf{k}-\mathbf{q}}^{\epsilon_n-\omega_m}\mathcal{G}_{\mathbf{k}'}^{\epsilon_n}\mathcal{G}_{\mathbf{k}'-\mathbf{q}}^{\epsilon_n-\omega_m}\mathcal{G}_{\mathbf{k}''-\mathbf{q}}^{\epsilon_n-\omega_m}\mathcal{G}_{\mathbf{k}''}^{\epsilon_n}, \\
\Sigma_\Gamma^{\mathrm{H}}(\mathbf{k}, \epsilon_n) &= \frac{1}{\beta}\sum_{\omega_m}\sum_{\mathbf{q}}\sum_{\mathbf{k}'}\sum_{\mathbf{k}''} V_{\mathbf{q}-\mathbf{k}'\to\mathbf{q}-\mathbf{k}''}^{\mathbf{k}'\to\mathbf{k}''} \Gamma(\mathbf{k}, \mathbf{k}', \omega_m)\Gamma(\mathbf{k}'', \mathbf{k}, \omega_m)\mathcal{G}_{\mathbf{q}-\mathbf{k}}^{\epsilon_n-\omega_m}\mathcal{G}_{\mathbf{k}'}^{\epsilon_n}\mathcal{G}_{\mathbf{k}''}^{\epsilon_n}\mathcal{G}_{\mathbf{q}-\mathbf{k}'}^{\epsilon_n-\omega_m}\mathcal{G}_{\mathbf{q}-\mathbf{k}''}^{\epsilon_n-\omega_m},
\end{aligned} \tag{S42}$$

where $1/\beta = k_B T$, $V$ stands for the interaction, $\Lambda$ for Diffison, and $\Gamma$ for Cooperon, as introduced as follows.

### B. Dynamically screened chiral interaction.

The bare interaction is described by the Hamiltonian

$$V_{ee} = \frac{1}{2}\sum_{\mathbf{k},\mathbf{k}',\mathbf{q}} v(q)(\phi^\dagger_{\mathbf{k}}\cdot\phi_{\mathbf{k}+\mathbf{q}})(\phi^\dagger_{\mathbf{k}'}\cdot\phi_{\mathbf{k}'-\mathbf{q}})c^\dagger_{\mathbf{k}'}c^\dagger_{\mathbf{k}}c_{\mathbf{k}+\mathbf{q}}c_{\mathbf{k}'-\mathbf{q}}, \tag{S43}$$

where the spinor[2] $\phi_{\mathbf{k}} = (a, -ie^{i\varphi}b)^T$, $\tan\varphi \equiv k_y/k_x$, $\mathbf{k}$ is the wave vector, $a \equiv \cos(\theta/2)$, $b \equiv \sin(\theta/2)$, and $\cos\theta \equiv \Delta/2E_F$. The interaction between Dirac fermions inherits the chiralities from $\phi_{\mathbf{k}}$[10]. $\mathbf{q}$ is the wave vector exchanged during the interaction-induced scattering, $q = |\mathbf{q}|$, and

$$v(q) \equiv \int \mathrm{d}^2\mathbf{r}\frac{e^{-i\mathbf{q}\cdot\mathbf{r}}}{4\pi\varepsilon_0\varepsilon_r|\mathbf{r}|} = \frac{e^2}{2\varepsilon_0\varepsilon_r q}, \tag{S44}$$

with $\varepsilon_0$ and $\varepsilon_r$ the vacuum and relative permittivities, respectively. In Fig. S2 (c), the bare interaction is renormalized into the dynamically screened interaction $V(\mathbf{q},\omega_m)$ under the disorder-dressed random phase approximation. $V^{\mathbf{k}'\to\mathbf{k}'-\mathbf{q}}_{\mathbf{k}''-\mathbf{q}\to\mathbf{k}''}$ in $\Sigma^{\mathrm{F}}_{\Lambda}$ reduces to $V^{\omega_m}_{\mathbf{q}}$ as $\mathbf{q}\to 0$, and

$$V^{\omega_m}_{\mathbf{q}} \equiv V(\mathbf{q},\omega_m) = \frac{v(q)}{1 - v(q)\Pi(\mathbf{q},\omega_m)}, \tag{S45}$$

where $\omega_m = 2\pi k_B T m/\hbar$ with $m \in \{0,1,2,...\}$ is bosonic Matsubara frequency, and the density response function[11]

$$\Pi(\mathbf{q},\omega_m) \approx -N_F\frac{Dq^2}{\omega_m + Dq^2}. \tag{S46}$$

For the interactions in $\Sigma^{\mathrm{H}}_{\Lambda}$, $\Sigma^{\mathrm{F}}_{\Gamma}$, and $\Sigma^{\mathrm{H}}_{\Gamma}$, we approximate that

$$V^{\mathbf{k}'\to\mathbf{k}''}_{\mathbf{q}-\mathbf{k}'\to\mathbf{q}-\mathbf{k}''} \approx \overline{V^{\omega_m=0}_{|\mathbf{k}-\mathbf{k}'|}}(\phi^\dagger_{-\mathbf{k}''}\cdot\phi_{-\mathbf{k}'})(\phi^\dagger_{\mathbf{k}''}\cdot\phi_{\mathbf{k}'}), \tag{S47}$$

where the overline means averaging over the momentum angles $\varphi$ and $\varphi'$ on the Fermi surface. From which, the screening factor is defined

$$F \equiv \frac{\overline{V^{\omega_m=0}_{|\mathbf{k}-\mathbf{k}'|}}}{V^{\omega_m=0}_{q=0}}, \tag{S48}$$

where $V^{\omega_m=0}_{q=0} = 1/N_F$ according to Eq. (S45). The evaluation of $F$ will be given in Sec. S3.

### C. Disorder scattering.

The Diffuson and Cooperon come from the disorder scattering by impurities. In this work, we only consider nonmagnetic impurities. The impurity potential is modeled as

$$U(\mathbf{r}) = \sum_i u_0^i\delta(\mathbf{r}-\mathbf{R}_i), \tag{S49}$$

where $\mathbf{R}_i$ are the positions of the random impurities. $u_0^i$ depicts the potential at $\mathbf{R}_i$. We assume short-range and delta-correlated disorder so that $\langle U(\mathbf{r})\rangle_{\mathrm{imp}} = 0$ and $\langle U(\mathbf{r})U(\mathbf{r}')\rangle_{\mathrm{imp}} \sim \delta(\mathbf{r}-\mathbf{r}')$, where $\langle ...\rangle_{\mathrm{imp}}$ means average over impurity configurations. The scattering matrix element can be found as $U_{\mathbf{k},\mathbf{k}'} \equiv \langle\psi_{\mathbf{r}}(\mathbf{k})|U(\mathbf{r})|\psi_{\mathbf{r}}(\mathbf{k}')\rangle$, where the wave function of the higher band of the Dirac model $\psi_{\mathbf{k}}(\mathbf{r}) = \phi_{\mathbf{k}}e^{i\mathbf{k}\cdot\mathbf{r}}/\sqrt{S}$ with $\phi_{\mathbf{k}}$ the spinor wavefunctin and $S$ is the area[2]. Under the Born approximation, the momentum relaxation time $\tau$ is found as

$$\begin{aligned} 1/\tau &\equiv (2\pi/\hbar)\sum_{\mathbf{k}'}\langle|U_{\mathbf{k},\mathbf{k}'}|^2\rangle_{\mathrm{imp}}\delta(\omega-\epsilon_{\mathbf{k}'}) \\ &= (2\pi/\hbar)N_F n_0 u_0^2(a^4+b^4), \end{aligned} \tag{S50}$$

where $n_0$ is the concentration of impurities and $u_0$ is the averaged scattering strength. We assume a dirty limit, in which the mean free path $\ell \equiv \sqrt{D\tau}$ is the shortest length scale, compared to the phase coherence length $\ell_\phi$, system size, magnetic length $\ell_B \equiv \sqrt{\hbar/4eB}$, and the thermal diffusion length $\ell_T \equiv \sqrt{D\hbar/2\pi k_B T}$.

### D. Diffuson and Cooperon.

The Diffuson and Cooperon can be found by their Bethe-Salpeter equations in Fig. S2 (c)

$$\begin{aligned} \Lambda_{\mathbf{k}_\alpha\mathbf{k}_\beta} &= \Lambda^0_{\mathbf{k}_\alpha\mathbf{k}_\beta} + \sum_{\mathbf{k}} \Lambda^0_{\mathbf{k}_\alpha\mathbf{k}} \mathcal{G}^{\epsilon_n}_{\mathbf{k}} \mathcal{G}^{\epsilon_n-\omega_m}_{\mathbf{k}-\mathbf{q}} \Lambda_{\mathbf{k}\mathbf{k}_\beta}, \\ \Gamma_{\mathbf{k}_\alpha\mathbf{k}_\beta} &= \Gamma^0_{\mathbf{k}_\alpha\mathbf{k}_\beta} + \sum_{\mathbf{k}} \Gamma^0_{\mathbf{k}_\alpha\mathbf{k}} \mathcal{G}^{\epsilon_n}_{\mathbf{k}} \mathcal{G}^{\epsilon_n-\omega_m}_{\mathbf{q}-\mathbf{k}} \Gamma_{\mathbf{k}\mathbf{k}_\beta}, \end{aligned} \tag{S51}$$

where $\mathbf{q} = \mathbf{k}_\alpha - \mathbf{k}_\beta$ in the Diffuson while $\mathbf{q} = \mathbf{k}_\alpha + \mathbf{k}_\beta$ in the Cooperon. The bare Diffuson and Cooperon are defined as the correction between the scattering matrix elements $\Lambda^0_{\mathbf{k}_\alpha\mathbf{k}_\beta} \equiv \langle U_{\mathbf{k}_\alpha,\mathbf{k}_\beta} U_{\mathbf{k}_\beta-\mathbf{q},\mathbf{k}_\alpha-\mathbf{q}}\rangle$ and $\Gamma^0_{\mathbf{k}_\alpha\mathbf{k}_\beta} \equiv \langle U_{\mathbf{k}_\alpha,\mathbf{k}_\beta} U_{\mathbf{q}-\mathbf{k}_\beta,\mathbf{q}-\mathbf{k}_\alpha}\rangle$. As $\mathbf{q} \to 0$,

$$\Lambda^0_{\mathbf{k}_\alpha\mathbf{k}_\beta} \approx \frac{\hbar}{2\pi N_F \tau}[d_1 + 2d_2\cos(\varphi_\alpha - \varphi_\beta)], \tag{S52}$$

with $d_1 = 1$, $d_2 = a^2b^2/(a^4+b^4)$, and

$$\Gamma^0_{\mathbf{k}_\alpha\mathbf{k}_\beta} = \frac{\hbar}{2\pi N_F \tau}[c_1 + c_2 e^{i(\varphi_\alpha-\varphi_\beta)} + c_3 e^{i2(\varphi_\alpha-\varphi_\beta)}], \tag{S53}$$

with $c_1 = a^4/(a^4+b^4)$, $c_2 = 2a^2b^2/(a^4+b^4)$, and $c_3 = b^4/(a^4+b^4)$. The kernels in the Diffusion and Cooperon have the same form in polar coordinates

$$\int \frac{kdk}{2\pi} \mathcal{G}^{\epsilon_n}_{\mathbf{k}} \mathcal{G}^{\epsilon_n-\omega_m}_{\pm(\mathbf{k}-\mathbf{q})} \approx \frac{2\pi N_F \tau}{\hbar} \frac{\theta(\epsilon_n(\omega_m - \epsilon_n))}{1 + \omega_m\tau + i\tau \mathbf{v}_F\cdot\mathbf{q}}. \tag{S54}$$

where $\theta$ is the step function, $\mathbf{q} = (q_x, q_y)$, and $\mathbf{v}_F \equiv v_F(\cos\varphi, \sin\varphi)$. We find the Diffuson and Cooperon take the forms

$$\begin{aligned} \Lambda(\mathbf{k},\mathbf{k}',\omega_m) &\approx \frac{\hbar}{2\pi N_F \tau^2} \frac{1}{\omega_m + D|\mathbf{k}-\mathbf{k}'|^2}, \\ \Gamma(\mathbf{k},\mathbf{k}',\omega_m) &\approx \frac{\hbar}{2\pi N_F \tau^2}\Big[\frac{1}{\omega_m + \Omega_0 + D_0|\mathbf{k}+\mathbf{k}'|^2} + \frac{e^{i(\varphi-\varphi')}}{\omega_m + \Omega_1 + D_1|\mathbf{k}+\mathbf{k}'|^2}\Big], \end{aligned} \tag{S55}$$

where $\mathbf{k}$ and $\mathbf{k}'$ are the wave vectors. The first term in $\Gamma$ is from the triplet Cooperon and the second term from the singlet Cooperon[9]. $\varphi$ ($\varphi'$) is the angle of the wave vector $\mathbf{k}$ ($\mathbf{k}'$). $\Omega_i$ and $D_i$ are the Cooperon gaps and diffusion coefficients of the Cooperons. At $\Delta/2E_F = 0$, $\Omega_1$ vanishes, then the singlet Cooperon diverges, leading to WAL; as $\Delta/2E_F \to 1$, $\Omega_0$ vanishes, then the triplet Cooperon diverges, leading to WL[2,8,9]. $\mathbf{k}+\mathbf{k}'$ in the Cooperon acquires a doubled Peierls's replacement in a magnetic field, giving rise to the magnetoconductivity.

### E. In magnetic field.

In the magnetoconductivity of the conventional 2DEG, besides the orbital effect on the Cooperons, the Zeeman effect can also enter the Hartree diagrams because of the spin degeneracy on the Fermi surface[5]. For the massive Dirac model, the only band on the Fermi surface is inactive to the in-plane Zeemen effect because of the gauge invariance, while the out-of-plane Zeeman is absorbed into $\Delta$ if the Dirac model corresponds to real spin. As a result, the orbital effect from Hartree-Cooperon self-energy dominates the magnetoconductivity. The perpendicular magnetic field changes the integral over the Cooperon momentum $q$ into the summation over the Landau levels (indexed by $\nu$)

$$\sum_{\mathbf{q}} \to \int_{\ell_\phi^{-2}}^{\ell^{-2}} \frac{d(q^2)}{4\pi} \to \frac{1}{4\pi}\frac{4eB}{\hbar}\sum_{\nu=\ell_B^2/\ell_\phi^2}^{\ell_B^2/\ell^2}, \tag{S56}$$

where $\ell$ is the mean free path, $\ell_\phi$ is the phase coherence length, and $\ell_B \equiv \sqrt{\hbar/4eB}$ is the magnetic scattering length. In the integrand, $q^2$ is quantized to $(\nu+1/2)/\ell_B^2$. In the dirty limit, $\ell \to 0$.

## S3. SCREENING FACTOR $F$.

The screening factor is defined [Eq. (S48)] as

$$F \equiv N_F \langle V(\mathbf{k}-\mathbf{k}',0)\rangle, \tag{S57}$$

where $\langle ...\rangle$ means the average of the interaction $V(\mathbf{k}-\mathbf{k}',\omega=0)$ over momenta $\mathbf{k}$ and $\mathbf{k}'$ on the Fermi surface, and using Eqs. (S44), (S45), and (S46)

$$V(\mathbf{k}-\mathbf{k}',0) \;=\; \frac{v(\mathbf{k}-\mathbf{k}')}{1-v(\mathbf{k}-\mathbf{k}')\Pi(\mathbf{k}-\mathbf{k}',0)}, \tag{S58}$$

with

$$v(\mathbf{k}-\mathbf{k}') = \frac{e^2}{2\varepsilon_0\varepsilon_r|\mathbf{k}-\mathbf{k}'|}, \quad \Pi(\mathbf{k}-\mathbf{k}',\omega=0) \approx -N_F\frac{D|\mathbf{k}-\mathbf{k}'|^2}{-i\omega+D|\mathbf{k}-\mathbf{k}'|^2}\bigg|_{\omega=0} = -N_F, \tag{S59}$$

where $\varepsilon_0$ is the vacuum permittivity and $\varepsilon_r$ is the relative permittivity of the material. Then

$$V(\mathbf{k}-\mathbf{k}',0) = \frac{\frac{e^2}{2\varepsilon_0\varepsilon_r}}{|\mathbf{k}-\mathbf{k}'|+1/\xi}, \tag{S60}$$

where we have defined the screening length $\xi$,

$$\frac{1}{\xi} \equiv \frac{e^2}{2\varepsilon_0\varepsilon_r}N_F = \frac{e^2}{2\varepsilon_0\varepsilon_r}\frac{E_F}{2\pi\gamma^2}. \tag{S61}$$

On the Fermi surface, $\mathbf{k} = k_F\cos\varphi$, $\mathbf{k}' = k_F\cos\varphi'$,

$$|\mathbf{k}-\mathbf{k}'|_{k_F} \;=\; \sqrt{k_F^2+k_F^2-2k_F^2\cos(\varphi-\varphi')} = \sqrt{2k_F^2[1-\cos(\varphi-\varphi')]} = 2k_F|\sin\frac{\varphi-\varphi'}{2}|, \tag{S62}$$

and

$$V(\mathbf{k}-\mathbf{k}',0)|_{k_F} = \frac{\frac{e^2}{2\varepsilon_0\varepsilon_r}}{2k_F|\sin\frac{\varphi-\varphi'}{2}|+1/\xi}. \tag{S63}$$

Then

$$\begin{aligned} F \;&\equiv\; N_F\frac{\int\frac{d\varphi}{2\pi}\int\frac{d\varphi'}{2\pi}\int\frac{kdk}{2\pi}\delta(k-k_F)\int\frac{k'dk'}{2\pi}\delta(k'-k_F)V(\mathbf{k}-\mathbf{k}',0)}{\int\frac{d\varphi}{2\pi}\int\frac{d\varphi'}{2\pi}\int\frac{\delta(k-k_F)kdk}{2\pi}\int\frac{\delta(k'-k_F)k'dk'}{2\pi}} = \frac{\int\frac{d\varphi}{2\pi}\int\frac{d\varphi'}{2\pi}(k_F/2\pi)^2\frac{\frac{e^2}{2\varepsilon_0\varepsilon_r}N_F}{2k_F|\sin\frac{\varphi-\varphi'}{2}|+1/\xi}}{(k_F/2\pi)^2} \\ &= \int\frac{d\varphi}{2\pi}\int\frac{d\varphi'}{2\pi}\frac{1/\xi}{2k_F|\sin\frac{\varphi-\varphi'}{2}|+1/\xi} = \int\frac{d\varphi}{2\pi}\int\frac{d\varphi'}{2\pi}\frac{1}{2k_F\xi|\sin\frac{\varphi-\varphi'}{2}|+1}. \end{aligned} \tag{S64}$$

Using

$$\int_0^{2\pi}\frac{d\varphi}{2\pi}\int_0^{2\pi}\frac{d\varphi'}{2\pi} \;=\; \int_0^{2\pi}\frac{d(\varphi+\varphi')}{2\pi}\int_0^{2\pi}\frac{d(\varphi-\varphi')}{2\pi}, \tag{S65}$$

we have

$$F \;=\; \int_0^{2\pi}\frac{d(\varphi+\varphi')}{2\pi}\int_0^{2\pi}\frac{d(\varphi-\varphi')}{2\pi}\frac{1}{2k_F\xi|\sin\frac{\varphi-\varphi'}{2}|+1} = \int_0^{2\pi}\frac{dx}{2\pi}\frac{1}{2k_F\xi\sin\frac{x}{2}+1}, \tag{S66}$$

where $x/2\in[0,\pi]$ so $|\sin(x/2)| = \sin(x/2)$. It can be shown that

$$0\le F \;=\; \int_0^{2\pi}\frac{dx}{2\pi}\frac{1}{2k_F\xi\sin\frac{x}{2}+1} \le \int_0^{2\pi}\frac{dx}{2\pi} = 1. \tag{S67}$$

In the limit $k_F\xi \to \infty$, $F = 0$; and in the limit $k_F\xi \to 0$, $F = 1$. The integral can be performed

$$F = \frac{2}{\pi}\frac{\arctan\sqrt{1/(2k_F\xi)^2 - 1}}{\sqrt{1-(2k_F\xi)^2}}, \tag{S68}$$

and

$$k_F\xi = \frac{k_F}{\frac{e^2}{2\varepsilon_0\varepsilon_r}N_F} = \frac{k_F}{\frac{e^2}{2\varepsilon_0\varepsilon_r}\frac{E_F}{2\pi\gamma^2}} = \frac{4\pi\varepsilon_0\varepsilon_r\gamma}{e^2}\frac{\gamma k_F}{E_F} = \frac{4\pi\varepsilon_0\varepsilon_r\gamma}{e^2}\sqrt{1-(\frac{\Delta}{2E_F})^2}. \tag{S69}$$

Notice that $\xi \propto \varepsilon_r$, which means that a larger $\varepsilon_r$, that is, a stronger screening of the electrostatic force by the lattice ions and valence electrons, leads to a longer $\xi$, that is, a weaker screening of the interaction between electrons. Back to the real space, after the normalization by disorders, the interaction becomes

$$V(r) = \frac{e^2}{4\pi\varepsilon_0\varepsilon_r r}\exp(-\frac{r}{\xi}) \propto \frac{1}{\varepsilon_r}\exp(-\frac{1}{\varepsilon_r}). \tag{S70}$$

As a function of the sheet carrier density $n = k_F^2/4\pi$,

$$k_F\xi = \frac{4\pi\varepsilon_0\varepsilon_r\gamma^2}{e^2}\frac{k_F}{E_F} = \frac{4\pi\varepsilon_0\varepsilon_r\gamma^2}{e^2}\frac{\sqrt{4\pi n}}{\sqrt{4\pi n\gamma^2 + (\frac{\Delta}{2})^2}} = \frac{4\pi\varepsilon_0\varepsilon_r\gamma}{e^2}\frac{\sqrt{4\pi n}}{\sqrt{4\pi n + (\frac{\Delta}{2\gamma})^2}}. \tag{S71}$$

Now we show the above integral of $F$,

$$F = \int_0^{2\pi}\frac{dx}{2\pi}\frac{1}{2k_F\xi\sin\frac{x}{2} + 1}. \tag{S72}$$

Let $x/2 \to x$ and $2k_F\xi = z \in [0,\infty)$, then

$$F = \int_0^{\pi}\frac{dx}{\pi}\frac{1}{z\sin x + 1}. \tag{S73}$$

Let $y = \tan(x/2)$, then $y \in [0,\infty)$, $\sin x = \frac{2y}{y^2+1}$, $dx = \frac{2}{y^2+1}dy$, and

$$F = \frac{2}{\pi}\int_0^{\infty} dy\frac{1}{y^2+2zy+1} = \frac{2}{\pi}\int_0^{\infty} dy\frac{1}{(y+z)^2+1-z^2}. \tag{S74}$$

It has three cases.

(1) If $1 - z^2 > 0$, that is, $z \in [0, 1)$,

$$\begin{aligned} F &= \frac{2}{\pi}\frac{1}{\sqrt{1-z^2}}\int_0^{\infty} d(\frac{y+z}{\sqrt{1-z^2}})\frac{1}{(\frac{y+z}{\sqrt{1-z^2}})^2+1} = \frac{2}{\pi}\frac{1}{\sqrt{1-z^2}}\arctan\frac{y+z}{\sqrt{1-z^2}}\Big|_0^{\infty} \\ &= \frac{2}{\pi}\frac{1}{\sqrt{1-z^2}}\left(\frac{\pi}{2} - \arctan\frac{z}{\sqrt{1-z^2}}\right) = \frac{2}{\pi}\frac{1}{\sqrt{1-z^2}}\left(\frac{\pi}{2} - \arctan\frac{1}{\sqrt{(1/z)^2-1}}\right). \end{aligned} \tag{S75}$$

Using $\pi/2 - \arctan(1/x)$=$\arctan(x)$ for $x > 0$,

$$F = \frac{2}{\pi}\frac{\arctan\sqrt{(1/z)^2-1}}{\sqrt{1-z^2}}, \quad z \in [0, 1). \tag{S76}$$

(2) If $1 - z^2 = 0$, that is, $z = 1$,

$$F = \frac{2}{\pi}\int_0^{\infty} dy\frac{1}{(y+1)^2} = -\frac{2}{\pi}\frac{1}{y+1}\Big|_0^{\infty} = \frac{2}{\pi}. \tag{S77}$$

Consider the limit $z \to 1$, where both the denominator and numerator goes to 0. Using L'Hôspital's rule

$$F = \frac{2}{\pi}\lim_{z\to 1}\frac{\arctan\sqrt{(1/z)^2-1}}{\sqrt{1-z^2}} = \frac{2}{\pi}\lim_{z\to 1}\frac{\frac{1}{1+(1/z)^2-1}\frac{(-2)z^{-3}}{2\sqrt{(1/z)^2-1}}}{\frac{-z}{\sqrt{1-z^2}}} = \frac{2}{\pi}\lim_{z\to 1}\frac{\frac{1}{(1/z)^2}\frac{z^{-2}}{\sqrt{1-z^2}}}{\frac{z}{\sqrt{1-z^2}}} = \frac{2}{\pi}\lim_{z\to 1}\frac{1}{z} = \frac{2}{\pi}. \tag{S78}$$

(3) If $z \in (1,\infty)$, that is, $1-z^2<0$,

$$F = \frac{2}{\pi}\int_0^\infty dy\frac{1}{(y+z)^2+1-z^2} = \frac{2}{\pi}\int_0^\infty dy\frac{1}{(y+z)^2-(z^2-1)} = \frac{2}{\pi}\frac{1}{\sqrt{z^2-1}}\int_0^\infty d(\frac{y+z}{\sqrt{z^2-1}})\frac{1}{(\frac{y+z}{\sqrt{z^2-1}})^2-1}$$
$$= \frac{2}{\pi}\frac{1}{\sqrt{z^2-1}}\int_{z/\sqrt{z^2-1}}^\infty dt\frac{1}{t^2-1} = \frac{1}{\pi}\frac{1}{\sqrt{z^2-1}}\int_{z/\sqrt{z^2-1}}^\infty dt\left(\frac{1}{t-1}-\frac{1}{t+1}\right)$$
$$= \frac{1}{\pi}\frac{1}{\sqrt{z^2-1}}\ln\frac{t-1}{t+1}\bigg|_{z/\sqrt{z^2-1}}^\infty = -\frac{1}{\pi}\frac{1}{\sqrt{z^2-1}}\ln\frac{\frac{z}{\sqrt{z^2-1}}-1}{\frac{z}{\sqrt{z^2-1}}+1} = \frac{1}{\pi}\frac{1}{\sqrt{z^2-1}}\ln\frac{z+\sqrt{z^2-1}}{z-\sqrt{z^2-1}}, \quad \text{(S79)}$$

so

$$F = \frac{1}{\pi}\frac{1}{\sqrt{z^2-1}}\ln\frac{1+\sqrt{1-(1/z)^2}}{1-\sqrt{1-(1/z)^2}}, \qquad z\in(1,\infty). \quad \text{(S80)}$$

Now we show the alternative expression, first

$$F = \frac{1}{\pi}\frac{1}{\sqrt{-1(1-z^2)}}\ln\frac{1+\sqrt{-1[(1/z)^2-1]}}{1-\sqrt{-1[(1/z)^2-1]}}. \quad \text{(S81)}$$

Suppose we can define $\sqrt{-1}=i$,

$$F = \frac{1}{\pi}\frac{1}{i\sqrt{1-z^2}}\ln\frac{1+i\sqrt{(1/z)^2-1}}{1-i\sqrt{(1/z)^2-1}} = \frac{i}{\pi}\frac{1}{\sqrt{1-z^2}}\ln\frac{i+\sqrt{(1/z)^2-1}}{i-\sqrt{(1/z)^2-1}}; \quad \text{(S82)}$$

or we can define $\sqrt{-1}=-i$, still the same expression

$$F = \frac{1}{\pi}\frac{1}{-i\sqrt{1-z^2}}\ln\frac{1-i\sqrt{(1/z)^2-1}}{1+i\sqrt{(1/z)^2-1}} = \frac{i}{\pi}\frac{1}{\sqrt{1-z^2}}\ln\frac{i+\sqrt{(1/z)^2-1}}{i-\sqrt{(1/z)^2-1}}. \quad \text{(S83)}$$

Now we use the property of complex functions (6.1.16(c), Page 371, G. B. Arfken and H. J. Weber, *Mathematical methods for physicists*, 4th. edition, Academic Press, 1995)

$$\arctan(z) = \frac{i}{2}\ln\frac{i+z}{i-z}, \quad \text{(S84)}$$

then

$$F = \frac{2}{\pi}\frac{\arctan\sqrt{(1/z)^2-1}}{\sqrt{1-z^2}}. \quad \text{(S85)}$$

This expression is valid regardless that $\sqrt{-1}\equiv\pm i$.

For the conventional 2DEG, the screening factor $F$ is corrected to $\frac{3}{4}\tilde{F}$, where the tilde comes from the interaction-induced correction to the disorder scattering and $-\frac{1}{4}$ from the second-order diagrams.[12] After the correction, the conductivity formula remains the same form and $\tilde{F}\approx 0.86F$ as $F\to 1$ and $\tilde{F}\approx F$ when $F\ll 1$. These corrections are then not urgent for the $Bi_2Se_3$-like topological insulators (where $F\ll 1$) but necessary for massive Dirac systems with much smaller relative permittivities.

## S4. CONDUCTIVITY FOR $\Delta/2E_F$ BETWEEN 0 AND 1.

See Fig. S3.

## S5. SLOPE OF $\sigma$ VS. $\ln T$.

### A. Experimental data of slope.

See Tab. S1 for the slope data extracted from the experiments.

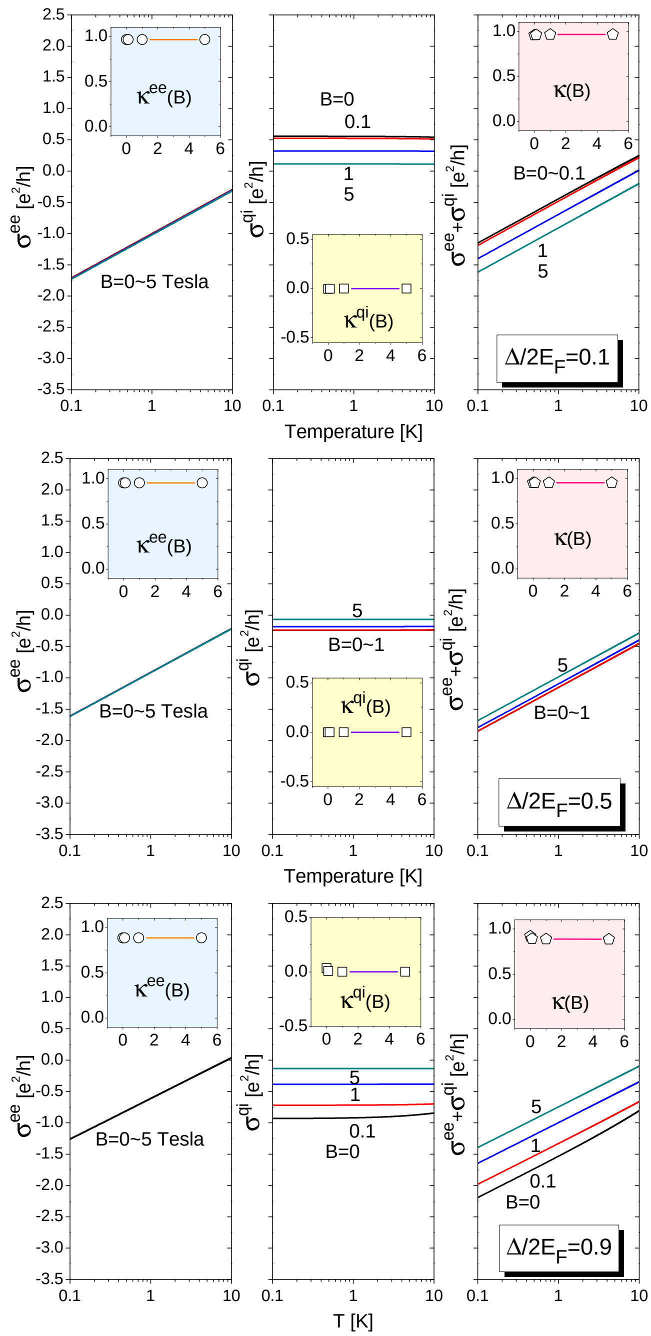


FIG. S3: The conductivity corrections from the quantum interference [$\sigma^{qi}$ in Eq. (2) of the main text] and the electron-electron interaction [$\sigma^{ee}$ in Eq. (3) of the main text] as functions of temperature $T$ under a perpendicular magnetic field $B$ for $\Delta/2E_F = 0.1, 0.5,$ and $0.9$. Insets show the slopes at $T = 1$ K as functions of $B$. $\kappa^{ee} \equiv (\pi h/e^2)\partial\sigma^{ee}/\partial \ln T$, $\kappa^{qi} \equiv (\pi h/e^2)\partial\sigma^{qi}/\partial \ln T$, and $\kappa = \kappa^{qi} + \kappa^{ee}$. The parameters are the same as those in Fig. 3 of the main text.

## B. Theory of slope.

In all the experiments[13–17], the conductivity $\sigma$ decreases logarithmically when lowering temperature $T$. This behavior is quantitatively described by the slope

$$\kappa \equiv \frac{\pi h}{e^2}\frac{\partial \sigma}{\partial \ln T}. \tag{S86}$$

TABLE S1: Slope in experiments. The slope $\kappa \equiv (\pi h/e^2)\partial\sigma/\partial \ln T$. $\sigma$ is the conductivity. The change of slope $\delta\kappa \equiv \kappa(B_c) - \kappa(0)$. $B_c$ (about 1 Tesla) is a critical magnetic field, beyond which the slope saturates. $n$ is the sheet carrier density. $n$ for C and D are converted from their cubic carrier densities.

| Experiment | A[13] | $B_1$[14] | $B_2$[14] | C[15] | D[16] | E[17] |
|---|---|---|---|---|---|---|
| Compound | $Bi_2Se_3$ | $Bi_2Se_3$ | $Pb_xBi_{2-x}Se_3$ | $Cu_xBi_{2-x}Se_3$ | $Bi_2Te_3$ | $Bi_2Te_3$ |
| n [$10^{12}$/cm$^2$] | 20e$^-$ | 102e$^-$ | 49.5e$^-$ | 6.72e$^-$ | 37h$^+$ | 120e$^-$ |
| Thickness [nm] | 10 | 45 | 45 | 80 | 65 | 4 |
| $\kappa(B=0)$ | 0.68 | 0.86 | 0.70 | 1.37 | 1.33 | 0.58 |
| $\kappa(B=0.2)$ | 0.8 | - | - | - | - | 0.89 |
| $\kappa(B=0.5)$ | - | - | - | - | - | 0.98 |
| $\kappa(B=1)$ | 0.8 | - | - | - | - | 1.04 |
| $\kappa(B=2)$ | 0.8 | 1.18 | 1.29 | 1.68 | - | 1.07 |
| $\kappa(B=3)$ | 0.8 | - | - | 1.66 | - | - |
| $\kappa(B=5)$ | 0.8 | - | - | 1.67 | 1.66 | 1.09 |
| $\delta\kappa$ | 0.12 | 0.32 | 0.58 | 0.30 | 0.33 | 0.51 |

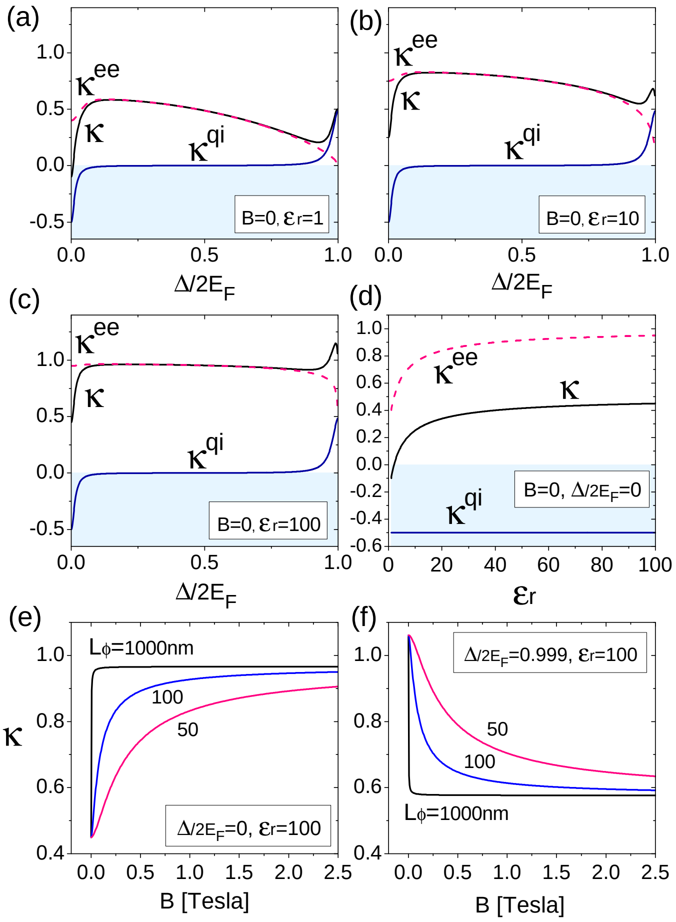


FIG. S4: The calculated slope of $\sigma$ vs. $\ln T$ of the massive Dirac fermions. $\kappa = \kappa^{qi} + \kappa^{ee}$, $\kappa^{qi} \equiv (\pi h/e^2)\partial\sigma^{qi}/\partial \ln T$, and $\kappa^{ee} \equiv (\pi h/e^2)\partial\sigma^{ee}/\partial \ln T$. $\sigma^{qi}$ and $\sigma^{ee}$ are the conductivity corrections from the quantum interference and electron-electron interaction, respectively. $\varepsilon_r$ is the relative permittivity. $\gamma = 3$ eVÅ. $\ell = 10$ nm. In (a)-(d), $B = 0$ Tesla and $\ell_\phi = 700$ nm. A negative $\kappa$ as large as $-0.1$ can be achieved for $\varepsilon_r < 2$ and $\Delta/2E_F < 0.01$. Otherwise, $\kappa$ is always positive. In (e)-(f), $\varepsilon_r = 100$ and $\Delta/2E_F = 0$. With decreasing $\ell_\phi$, the change of $\kappa$ with $B$ becomes less prompt, showing an increasing $B_\phi \equiv \hbar/4e\ell_\phi^2$. $B_\phi$ is the critical magnetic field beyond which the quantum interference is destroyed.

Then the observed $\kappa$ is positive. The slope is mainly determined by the electron-electron interaction and quantum interference $\kappa = \kappa^{ee} + \kappa^{qi}$. From $\sigma^{qi}$ (Eq. S11) and $\sigma^{ee}$ (Eq. S15),

$$\begin{aligned} \kappa^{qi} &= \alpha p, \\ \kappa^{ee} &\approx 1 - (\eta_\Lambda + \eta_\Gamma)F, \end{aligned} \tag{S87}$$

where we neglect the last term of $\sigma^{ee}$ for $F \ll 1$. There are three limits:

(1) In a strong magnetic field ($B \gg B_\phi$), $\sigma^{qi} = 0$, the slope is solely determined by $\kappa^{ee}$ as

$$\kappa^{B \gg B_\phi} = \kappa^{ee} = 1 - \eta_\Lambda F, \tag{S88}$$

which is always positive because $\eta_\Lambda \in [1/2, 1]$, $\eta_\Gamma \in [1/4, 0]$ (see Fig. S1), and $F \in [0, 1]$ according to Eq. (S67). The critical magnetic field $B_\phi$ is determined by $B_\phi = \hbar/4e\ell_\phi^2$. A shorter $\ell_\phi$ gives a larger $B_\phi$. Figures S4 **e** and **f** show that $\kappa$ saturates rapidly with increasing magnetic field if the phase coherence length is long (e.g., 1 $\mu$m). The rapid saturation of $\kappa$ can be slowed by decreasing $\ell_\phi$.

In other two limits, $B \ll B_\phi$, the slope is given by

$$\kappa^{B \ll B_\phi} = \kappa^{ee} + \kappa^{qi} = 1 - (\eta_\Lambda + \eta_\Gamma)F + \alpha p, \tag{S89}$$

where $p$=1 if the electron-electron interaction is the decoherence source in two-dimensional disordered metals[5].

(2) In the limit $B \ll B_\phi$ and $\Delta/2E_F \to 1$, $\alpha p \to 1/2$ because $\alpha \to 1/2$; while $\kappa^{ee} \to 1 - F$ is always positive, then the slope is also always positive.

(3) In the limit $B \ll B_\phi$ and $\Delta/2E_F$=0, $\kappa^{ee} = 1 - 3F/4 \in [1/4, 1]$; while $\alpha$=$-1/2$, so $\alpha p$=$-1/2$. Therefore, for $B \ll B_\phi$ and $\Delta/2E_F \sim 0$, we expect a negative $\kappa$ when $\kappa^{ee}$<1/2. Because $\eta_\Lambda$, $\eta_\Gamma$, and $F$ in $\kappa^{ee}$ are functions of $\Delta/2E_F$ and $\gamma\varepsilon_r$, which then determine the sign of $\kappa$. Figure S4 shows $\kappa$, $\kappa^{ee}$ and $\kappa^{qi}$ as functions of $\Delta/2E_F$ and $\varepsilon_r$ for a fixed $\gamma$. For $\gamma = 3$ eVÅ (comparable with those in topological insulators), a negative $\kappa$ as large as $-0.1$ can be achieved for $\varepsilon_r < 2$ and $\Delta/2E_F < 0.01$. Otherwise, the slope is always positive, consistent with the experiments[13–17].

---


[1] N. H. Shon and T. Ando, J. Phys. Soc. Jpn.**67**, 2421 (1998).
[2] H. Z. Lu, J. Shi, and S. Q. Shen, Phys. Rev. Lett. **107**, 076801 (2011).
[3] B. L. Altshuler and A. G. Aronov, in *Electron-electron interactions in disordered systems* edited by A. L. Efros and M. Pollak (North-Holland, Amsterdam, 1985).
[4] H. Fukuyama, in *Electron-electron interactions in disordered systems* edited by A. L. Efros and M. Pollak (North-Holland, Amsterdam, 1985).
[5] P. A. Lee, and T. V. Ramakrishnan, Rev. Mod. Phys. **57**, 287 (1985).
[6] E. McCann, K. Kechedzhi, V. I. Fal'ko, H. Suzuura, T. Ando, and B. L. Altshuler, Phys. Rev. Lett. **97**, 146805 (2006).
[7] S. Hikami, A. Larkin, and Y. Nagaoka, Prog. Theor. Phys. **63**, 707 (1980).
[8] H. Z. Lu and S. Q. Shen, Phys. Rev. B **84**, 125138 (2011).
[9] W. Y. Shan, H. Z. Lu, and S. Q. Shen, Phys. Rev. B **86**, 125303 (2012).
[10] T. Ando, J. Phys. Soc. Jpn. **75**, 074716 (2006).
[11] D. Vollhardt and P. Wolfle, Phys. Rev. B **22**, 4666 (1980).
[12] A. M. Finkel'shteĭn, Sov. Phys. JETP **57**, 97 (1983).
[13] J. Chen, X. Y. He, K. H. Wu, Z. Q. Ji, L. Lu, J. R. Shi, J. H. Smet, and Y. Q. Li, Phys. Rev. B **83**, 241304(R) (2011).
[14] J. Wang, A. M. DaSilva, C. Z. Chang, K. He, J. K. Jain, N. Samarth, X. C. Ma, Q. K. Xue, and M. H. W. Chan, Phys. Rev. B **83**, 245438 (2011).
[15] Y. Takagaki, B. Jenichen, U. Jahn, M. Ramsteiner, and K. J. Friedland, Phys. Rev. B **85**, 115314 (2012).
[16] S. P. Chiu and J. J. Lin, Phys. Rev. B **87**, 035122 (2013).
[17] A. Roy, S. Guchhait, S. Sonde, R. Dey, T. Pramanik, A. Rai, H. C. P. Movva, L. Colombo, and S. K. Banerjee, Appl. Phys. Lett. **102**, 163118 (2013).
